# Supplementary material for: BC Cassiopeiae: First Detection of IW And-Type Phenomenon Among Post-Eruption Novae
Source: arXiv:2009.12993 ancillary file (2020-09-28)
Supplement: Supplementary file 1 [file si.pdf]

doi: 10.1093/pasj/

# Supplementary Information to BC Cassiopeiae: First Detection of IW And-Type Phenomenon Among Post-Eruption Novae

**T. Kato and N. Kojiguchi**

Received 0 0; Accepted 0 0

## Abstract

## E-section 1 Reliability of the ZTF data

To check the reliability of the ZTF data for analysis of light curves of cataclysmic variables, we obtained light curves of two stars close to BC Cas (figure 1). These stars were selected from comparison stars listed in Henden and Honeycutt (1997). Although there were a few outlier points (probably caused by noise), the constancy of these comparison stars was confirmed. The resultant constancy confirmed the reliability of the ZTF data in discussing light curves of dwarf novae.

We also examined the phased light curve of WZ Sge, an eclipsing dwarf nova (figure 2). The resultant phased light curve is sufficient to confirm the reliability of the ZTF data in analyzing short-term variations, although this type of analysis was not made in this paper.

## E-section 2 Data of BC Cas from ZTF observations

| BJD−2400000 | Mag | Magerr | Filter | Obs code |
|---|---|---|---|---|
| 58230.003076 | 18.004 | 0.033 | zg | ZTF |
| 58232.999829 | 18.168 | 0.036 | zg | ZTF |
| 58246.982640 | 18.239 | 0.037 | zg | ZTF |
| 58247.984101 | 17.991 | 0.033 | zg | ZTF |
| 58252.963501 | 18.063 | 0.034 | zg | ZTF |
| 58255.928272 | 17.976 | 0.033 | zg | ZTF |
| 58258.984918 | 17.986 | 0.033 | zg | ZTF |
| 58259.929166 | 18.082 | 0.035 | zg | ZTF |
| 58262.974351 | 17.982 | 0.033 | zg | ZTF |
| 58263.963083 | 17.922 | 0.032 | zg | ZTF |
| 58267.965880 | 18.160 | 0.036 | zg | ZTF |
| 58268.965553 | 18.093 | 0.035 | zg | ZTF |
| 58269.970738 | 18.171 | 0.036 | zg | ZTF |
| 58270.967705 | 17.951 | 0.033 | zg | ZTF |
| 58272.930193 | 17.840 | 0.031 | zg | ZTF |
| 58273.965486 | 17.879 | 0.032 | zg | ZTF |
| 58274.918114 | 17.968 | 0.033 | zg | ZTF |
| 58276.905297 | 17.941 | 0.032 | zg | ZTF |
| 58277.946437 | 17.908 | 0.032 | zg | ZTF |
| 58278.933618 | 17.948 | 0.032 | zg | ZTF |

© 0000. Astronomical Society of Japan.

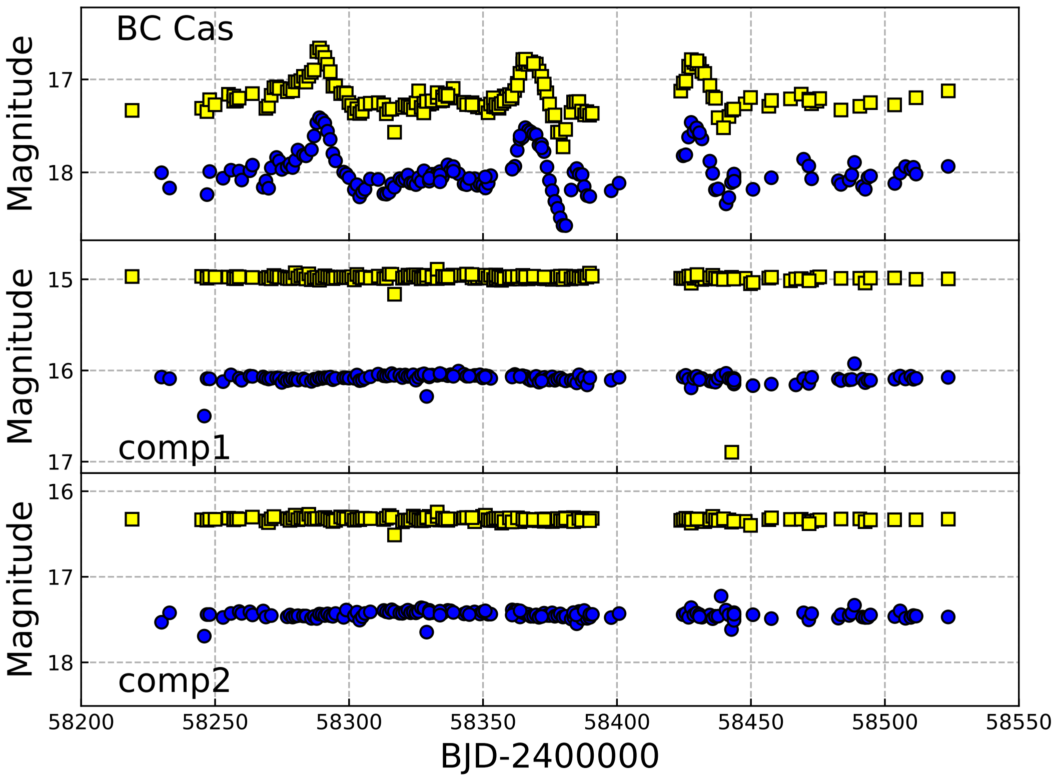


**E-figure 1.** Light curves of BC Cas and two comparison stars from the ZTF observations. The filled squares and circles represent $r$ and $g$ observations, respectively. The Coordinations of comp1 (Gaia DR2 2011556424241343744) and comp2 (Gaia DR2 2011649092455352192) are $23^{\rm h}50^{\rm m}59^{\rm s}.946$ $+60^{\circ}18'54''.38$ and $23^{\rm h}51^{\rm m}22^{\rm s}.313$ $+60^{\circ}17'10''.07$, respectively.

| BJD−2400000 | Mag | Magerr | Filter | Obs code |
|---|---|---|---|---|
| 58279.953579 | 17.869 | 0.031 | zg | ZTF |
| 58280.924511 | 17.760 | 0.030 | zg | ZTF |
| 58282.925939 | 17.814 | 0.031 | zg | ZTF |
| 58283.924813 | 17.822 | 0.031 | zg | ZTF |
| 58285.949070 | 17.756 | 0.030 | zg | ZTF |
| 58286.954533 | 17.609 | 0.028 | zg | ZTF |
| 58287.930689 | 17.466 | 0.027 | zg | ZTF |
| 58288.930145 | 17.412 | 0.026 | zg | ZTF |
| 58289.921604 | 17.435 | 0.026 | zg | ZTF |
| 58290.951688 | 17.471 | 0.027 | zg | ZTF |
| 58291.952929 | 17.557 | 0.028 | zg | ZTF |
| 58292.953788 | 17.645 | 0.029 | zg | ZTF |
| 58293.951847 | 17.798 | 0.030 | zg | ZTF |
| 58294.956527 | 17.876 | 0.031 | zg | ZTF |

| BJD−2400000 | Mag | Magerr | Filter | Obs code |
|---|---|---|---|---|
| 58297.969527 | 17.997 | 0.033 | zg | ZTF |
| 58298.970111 | 18.018 | 0.034 | zg | ZTF |
| 58299.968694 | 18.056 | 0.034 | zg | ZTF |
| 58301.969841 | 18.186 | 0.036 | zg | ZTF |
| 58302.950079 | 18.133 | 0.035 | zg | ZTF |
| 58303.943060 | 18.264 | 0.038 | zg | ZTF |
| 58304.944434 | 18.212 | 0.037 | zg | ZTF |
| 58305.954871 | 18.182 | 0.036 | zg | ZTF |
| 58307.949576 | 18.072 | 0.034 | zg | ZTF |
| 58310.864565 | 18.076 | 0.034 | zg | ZTF |
| 58312.965389 | 18.230 | 0.037 | zg | ZTF |
| 58313.948443 | 18.234 | 0.037 | zg | ZTF |
| 58314.965399 | 18.216 | 0.037 | zg | ZTF |
| 58315.926368 | 18.125 | 0.035 | zg | ZTF |

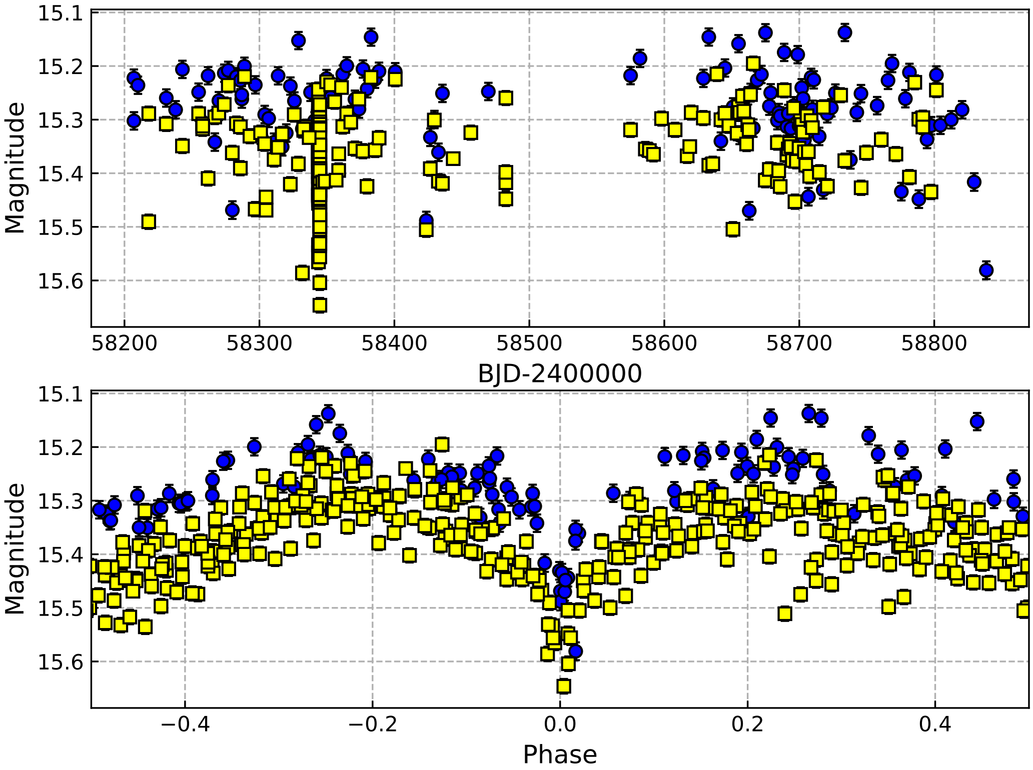


**E-figure 2.** Light curve and Phase-binned profile of WZ Sge from the ZTF observations. The filled squares and circles represent $r$ and $g$ observations, respectively. Phase-binned profile is based on the orbital ephemeris giving the heliocentric Julian dates of mid-eclipse, $T = 2437547.72845(3) + 0.0566878455(7) * E$ (Robinson et al. 1978).

| BJD−2400000 | Mag | Magerr | Filter | Obs code |
|---|---|---|---|---|
| 58316.907755 | 18.160 | 0.036 | zg | ZTF |
| 58318.925499 | 18.067 | 0.034 | zg | ZTF |
| 58319.906284 | 18.088 | 0.035 | zg | ZTF |
| 58320.957780 | 18.071 | 0.034 | zg | ZTF |
| 58321.932883 | 18.028 | 0.034 | zg | ZTF |
| 58322.946530 | 18.114 | 0.035 | zg | ZTF |
| 58323.954493 | 18.113 | 0.035 | zg | ZTF |
| 58324.952827 | 18.131 | 0.035 | zg | ZTF |
| 58325.926842 | 18.058 | 0.034 | zg | ZTF |
| 58326.964969 | 18.097 | 0.035 | zg | ZTF |
| 58327.972771 | 17.983 | 0.033 | zg | ZTF |
| 58329.979554 | 18.085 | 0.035 | zg | ZTF |
| 58330.973234 | 18.020 | 0.034 | zg | ZTF |
| 58332.949691 | 18.009 | 0.033 | zg | ZTF |

| BJD−2400000 | Mag | Magerr | Filter | Obs code |
|---|---|---|---|---|
| 58333.944980 | 17.992 | 0.033 | zg | ZTF |
| 58334.820447 | 18.052 | 0.034 | zg | ZTF |
| 58336.826117 | 17.919 | 0.032 | zg | ZTF |
| 58337.890541 | 17.978 | 0.033 | zg | ZTF |
| 58338.899731 | 17.938 | 0.032 | zg | ZTF |
| 58340.859726 | 18.015 | 0.033 | zg | ZTF |
| 58342.912202 | 18.124 | 0.035 | zg | ZTF |
| 58343.912999 | 18.132 | 0.035 | zg | ZTF |
| 58346.844133 | 18.067 | 0.034 | zg | ZTF |
| 58347.845900 | 18.139 | 0.035 | zg | ZTF |
| 58348.863976 | 18.124 | 0.035 | zg | ZTF |
| 58349.887573 | 18.136 | 0.035 | zg | ZTF |
| 58350.933161 | 18.168 | 0.036 | zg | ZTF |
| 58351.937774 | 18.117 | 0.035 | zg | ZTF |

| BJD−2400000 | Mag | Magerr | Filter | Obs code |
|---|---|---|---|---|
| 58352.890764 | 18.035 | 0.034 | zg | ZTF |
| 58360.911447 | 17.961 | 0.033 | zg | ZTF |
| 58361.888994 | 17.934 | 0.032 | zg | ZTF |
| 58362.763144 | 17.763 | 0.030 | zg | ZTF |
| 58363.810682 | 17.644 | 0.029 | zg | ZTF |
| 58364.763481 | 17.623 | 0.028 | zg | ZTF |
| 58365.802973 | 17.519 | 0.027 | zg | ZTF |
| 58366.910929 | 17.548 | 0.028 | zg | ZTF |
| 58367.814707 | 17.564 | 0.028 | zg | ZTF |
| 58368.872173 | 17.586 | 0.028 | zg | ZTF |
| 58369.819749 | 17.594 | 0.028 | zg | ZTF |
| 58370.862108 | 17.705 | 0.029 | zg | ZTF |
| 58371.847566 | 17.697 | 0.029 | zg | ZTF |
| 58372.785441 | 17.776 | 0.030 | zg | ZTF |
| 58373.874675 | 17.942 | 0.032 | zg | ZTF |
| 58374.785382 | 18.088 | 0.035 | zg | ZTF |
| 58375.805133 | 18.196 | 0.036 | zg | ZTF |
| 58376.806618 | 18.311 | 0.039 | zg | ZTF |
| 58377.849968 | 18.387 | 0.040 | zg | ZTF |
| 58378.828708 | 18.489 | 0.042 | zg | ZTF |
| 58379.846916 | 18.570 | 0.044 | zg | ZTF |
| 58380.871848 | 18.572 | 0.044 | zg | ZTF |
| 58382.906790 | 18.190 | 0.036 | zg | ZTF |
| 58383.930446 | 17.997 | 0.033 | zg | ZTF |
| 58384.968130 | 17.959 | 0.033 | zg | ZTF |
| 58385.866630 | 18.021 | 0.034 | zg | ZTF |
| 58386.992671 | 18.024 | 0.034 | zg | ZTF |
| 58387.757856 | 18.153 | 0.036 | zg | ZTF |
| 58388.865260 | 18.250 | 0.037 | zg | ZTF |
| 58389.851063 | 18.259 | 0.038 | zg | ZTF |
| 58397.854563 | 18.198 | 0.036 | zg | ZTF |
| 58400.780347 | 18.115 | 0.035 | zg | ZTF |
| 58424.690332 | 17.821 | 0.031 | zg | ZTF |
| 58425.682686 | 17.811 | 0.031 | zg | ZTF |
| 58426.717260 | 17.620 | 0.028 | zg | ZTF |
| 58427.690075 | 17.462 | 0.027 | zg | ZTF |
| 58428.686118 | 17.562 | 0.028 | zg | ZTF |
| 58429.728988 | 17.521 | 0.027 | zg | ZTF |
| 58430.762991 | 17.582 | 0.028 | zg | ZTF |
| 58431.728822 | 17.640 | 0.029 | zg | ZTF |
| 58434.657908 | 17.879 | 0.032 | zg | ZTF |

| BJD−2400000 | Mag | Magerr | Filter | Obs code |
|---|---|---|---|---|
| 58435.722160 | 18.010 | 0.033 | zg | ZTF |
| 58436.737234 | 18.188 | 0.036 | zg | ZTF |
| 58437.742353 | 18.178 | 0.036 | zg | ZTF |
| 58440.724418 | 18.339 | 0.039 | zg | ZTF |
| 58441.751940 | 18.271 | 0.038 | zg | ZTF |
| 58442.749242 | 18.110 | 0.035 | zg | ZTF |
| 58450.763399 | 18.182 | 0.036 | zg | ZTF |
| 58457.619280 | 18.058 | 0.034 | zg | ZTF |
| 58469.659297 | 17.858 | 0.031 | zg | ZTF |
| 58471.606554 | 17.931 | 0.032 | zg | ZTF |
| 58472.659130 | 18.069 | 0.034 | zg | ZTF |
| 58482.640223 | 18.090 | 0.035 | zg | ZTF |
| 58483.614336 | 18.129 | 0.035 | zg | ZTF |
| 58486.658149 | 18.083 | 0.035 | zg | ZTF |
| 58487.661530 | 18.027 | 0.034 | zg | ZTF |
| 58488.656173 | 17.893 | 0.032 | zg | ZTF |
| 58491.655076 | 18.150 | 0.036 | zg | ZTF |
| 58492.680017 | 18.182 | 0.036 | zg | ZTF |
| 58493.677633 | 18.055 | 0.034 | zg | ZTF |
| 58494.642796 | 18.039 | 0.034 | zg | ZTF |
| 58503.698429 | 18.119 | 0.035 | zg | ZTF |
| 58505.678264 | 18.007 | 0.033 | zg | ZTF |
| 58507.699069 | 17.937 | 0.032 | zg | ZTF |
| 58509.678232 | 17.965 | 0.033 | zg | ZTF |
| 58510.655813 | 17.945 | 0.032 | zg | ZTF |
| 58511.637733 | 18.018 | 0.034 | zg | ZTF |
| 58523.624596 | 17.936 | 0.032 | zg | ZTF |
| 58607.975954 | 17.939 | 0.032 | zg | ZTF |
| 58618.931379 | 17.558 | 0.028 | zg | ZTF |
| 58638.947854 | 18.014 | 0.033 | zg | ZTF |
| 58639.943944 | 17.987 | 0.033 | zg | ZTF |
| 58640.954052 | 18.029 | 0.034 | zg | ZTF |
| 58641.950734 | 17.899 | 0.032 | zg | ZTF |
| 58642.921652 | 17.985 | 0.033 | zg | ZTF |
| 58643.951681 | 17.793 | 0.030 | zg | ZTF |
| 58644.951386 | 17.932 | 0.032 | zg | ZTF |
| 58645.952412 | 17.917 | 0.032 | zg | ZTF |
| 58646.952558 | 17.971 | 0.033 | zg | ZTF |
| 58647.855270 | 18.020 | 0.034 | zg | ZTF |
| 58648.947598 | 18.000 | 0.033 | zg | ZTF |
| 58649.882952 | 18.104 | 0.035 | zg | ZTF |

| BJD−2400000 | Mag | Magerr | Filter | Obs code |
|---|---|---|---|---|
| 58650.973058 | 18.086 | 0.035 | zg | ZTF |
| 58652.965140 | 17.906 | 0.032 | zg | ZTF |
| 58653.886769 | 17.868 | 0.031 | zg | ZTF |
| 58657.972474 | 17.851 | 0.031 | zg | ZTF |
| 58663.964733 | 17.846 | 0.031 | zg | ZTF |
| 58665.969803 | 17.800 | 0.030 | zg | ZTF |
| 58666.972946 | 17.826 | 0.031 | zg | ZTF |
| 58667.953994 | 17.877 | 0.031 | zg | ZTF |
| 58668.955090 | 17.879 | 0.032 | zg | ZTF |
| 58669.954901 | 17.920 | 0.032 | zg | ZTF |
| 58670.927801 | 17.925 | 0.032 | zg | ZTF |
| 58673.850797 | 17.875 | 0.031 | zg | ZTF |
| 58680.973167 | 17.633 | 0.028 | zg | ZTF |
| 58683.968269 | 17.955 | 0.033 | zg | ZTF |
| 58686.969565 | 17.748 | 0.030 | zg | ZTF |
| 58690.945154 | 17.936 | 0.032 | zg | ZTF |
| 58696.920073 | 17.967 | 0.033 | zg | ZTF |
| 58706.924059 | 17.887 | 0.032 | zg | ZTF |
| 58709.972203 | 17.988 | 0.033 | zg | ZTF |
| 58712.966893 | 18.015 | 0.033 | zg | ZTF |
| 58727.890400 | 17.777 | 0.030 | zg | ZTF |
| 58730.816925 | 17.995 | 0.033 | zg | ZTF |
| 58733.949809 | 18.148 | 0.036 | zg | ZTF |
| 58736.970250 | 18.060 | 0.034 | zg | ZTF |
| 58739.995223 | 17.957 | 0.033 | zg | ZTF |
| 58743.910175 | 17.995 | 0.033 | zg | ZTF |
| 58747.815220 | 17.824 | 0.031 | zg | ZTF |
| 58750.869150 | 17.600 | 0.028 | zg | ZTF |
| 58754.789670 | 17.415 | 0.026 | zg | ZTF |
| 58760.864346 | 17.390 | 0.026 | zg | ZTF |
| 58763.885728 | 17.434 | 0.026 | zg | ZTF |
| 58764.687144 | 17.495 | 0.027 | zg | ZTF |
| 58765.687844 | 17.458 | 0.027 | zg | ZTF |
| 58766.686415 | 17.690 | 0.029 | zg | ZTF |
| 58767.683954 | 17.876 | 0.031 | zg | ZTF |
| 58768.684559 | 17.949 | 0.032 | zg | ZTF |
| 58769.684504 | 18.013 | 0.033 | zg | ZTF |
| 58770.684563 | 18.254 | 0.037 | zg | ZTF |
| 58771.684795 | 18.089 | 0.035 | zg | ZTF |
| 58772.685200 | 18.060 | 0.034 | zg | ZTF |
| 58774.683749 | 17.967 | 0.033 | zg | ZTF |
| 58775.683850 | 17.976 | 0.033 | zg | ZTF |
| 58776.683093 | 17.982 | 0.033 | zg | ZTF |
| 58777.683562 | 17.933 | 0.032 | zg | ZTF |
| 58778.683764 | 17.940 | 0.032 | zg | ZTF |
| 58779.683583 | 17.982 | 0.033 | zg | ZTF |
| 58781.683079 | 17.978 | 0.033 | zg | ZTF |
| 58782.681911 | 17.994 | 0.033 | zg | ZTF |
| 58783.682964 | 17.933 | 0.032 | zg | ZTF |
| 58785.682660 | 17.947 | 0.032 | zg | ZTF |
| 58786.691453 | 17.954 | 0.033 | zg | ZTF |
| 58787.681426 | 17.989 | 0.033 | zg | ZTF |
| 58788.682346 | 18.038 | 0.034 | zg | ZTF |
| 58789.682757 | 18.003 | 0.033 | zg | ZTF |
| 58790.772066 | 17.999 | 0.033 | zg | ZTF |
| 58791.784106 | 17.944 | 0.032 | zg | ZTF |
| 58793.652328 | 17.858 | 0.031 | zg | ZTF |
| 58793.683011 | 17.865 | 0.031 | zg | ZTF |
| 58794.683891 | 17.879 | 0.032 | zg | ZTF |
| 58795.673820 | 17.931 | 0.032 | zg | ZTF |
| 58796.680173 | 17.953 | 0.033 | zg | ZTF |
| 58797.678492 | 17.989 | 0.033 | zg | ZTF |
| 58798.621926 | 17.984 | 0.033 | zg | ZTF |
| 58798.661347 | 18.034 | 0.034 | zg | ZTF |
| 58800.685399 | 17.896 | 0.032 | zg | ZTF |
| 58801.681758 | 17.961 | 0.033 | zg | ZTF |
| 58803.687250 | 17.740 | 0.030 | zg | ZTF |
| 58804.686847 | 17.805 | 0.031 | zg | ZTF |
| 58805.683677 | 17.843 | 0.031 | zg | ZTF |
| 58811.689935 | 17.677 | 0.029 | zg | ZTF |
| 58812.638900 | 17.604 | 0.028 | zg | ZTF |
| 58814.622602 | 17.251 | 0.025 | zg | ZTF |
| 58819.699805 | 17.283 | 0.025 | zg | ZTF |
| 58820.678127 | 17.243 | 0.025 | zg | ZTF |
| 58820.706320 | 17.313 | 0.025 | zg | ZTF |
| 58828.602628 | 17.416 | 0.026 | zg | ZTF |
| 58829.617561 | 17.454 | 0.027 | zg | ZTF |
| 58831.617936 | 17.819 | 0.031 | zg | ZTF |
| 58833.637381 | 17.865 | 0.031 | zg | ZTF |
| 58836.614046 | 18.003 | 0.033 | zg | ZTF |
| 58839.625831 | 17.967 | 0.033 | zg | ZTF |
| 58219.011843 | 17.333 | 0.020 | zr | ZTF |

| BJD−2400000 | Mag | Magerr | Filter | Obs code |
|---|---|---|---|---|
| 58244.982847 | 17.311 | 0.020 | zr | ZTF |
| 58246.947674 | 17.346 | 0.020 | zr | ZTF |
| 58247.966126 | 17.219 | 0.019 | zr | ZTF |
| 58249.978854 | 17.273 | 0.020 | zr | ZTF |
| 58254.986030 | 17.160 | 0.019 | zr | ZTF |
| 58256.923653 | 17.235 | 0.020 | zr | ZTF |
| 58256.979569 | 17.179 | 0.019 | zr | ZTF |
| 58257.920783 | 17.232 | 0.020 | zr | ZTF |
| 58257.967393 | 17.218 | 0.019 | zr | ZTF |
| 58258.952660 | 17.202 | 0.019 | zr | ZTF |
| 58263.913267 | 17.153 | 0.019 | zr | ZTF |
| 58268.950379 | 17.312 | 0.020 | zr | ZTF |
| 58269.924833 | 17.287 | 0.020 | zr | ZTF |
| 58270.924752 | 17.171 | 0.019 | zr | ZTF |
| 58271.946639 | 17.090 | 0.019 | zr | ZTF |
| 58272.962301 | 17.081 | 0.019 | zr | ZTF |
| 58273.924709 | 17.097 | 0.019 | zr | ZTF |
| 58276.946768 | 17.132 | 0.019 | zr | ZTF |
| 58277.929758 | 17.100 | 0.019 | zr | ZTF |
| 58278.968979 | 17.122 | 0.019 | zr | ZTF |
| 58279.906471 | 17.025 | 0.018 | zr | ZTF |
| 58280.868953 | 17.027 | 0.018 | zr | ZTF |
| 58281.966881 | 17.013 | 0.018 | zr | ZTF |
| 58282.967457 | 16.967 | 0.018 | zr | ZTF |
| 58283.885460 | 17.029 | 0.018 | zr | ZTF |
| 58284.969698 | 16.965 | 0.018 | zr | ZTF |
| 58285.905886 | 16.924 | 0.018 | zr | ZTF |
| 58286.974244 | 16.898 | 0.018 | zr | ZTF |
| 58287.970911 | 16.700 | 0.017 | zr | ZTF |
| 58288.969302 | 16.662 | 0.017 | zr | ZTF |
| 58289.975739 | 16.706 | 0.017 | zr | ZTF |
| 58290.974676 | 16.764 | 0.017 | zr | ZTF |
| 58291.970233 | 16.838 | 0.017 | zr | ZTF |
| 58292.970166 | 16.917 | 0.018 | zr | ZTF |
| 58293.971315 | 17.073 | 0.019 | zr | ZTF |
| 58294.970926 | 17.068 | 0.019 | zr | ZTF |
| 58296.863718 | 17.152 | 0.019 | zr | ZTF |
| 58297.932754 | 17.144 | 0.019 | zr | ZTF |
| 58298.945839 | 17.151 | 0.019 | zr | ZTF |
| 58299.925485 | 17.249 | 0.020 | zr | ZTF |
| 58300.927911 | 17.280 | 0.020 | zr | ZTF |
| 58301.951310 | 17.361 | 0.020 | zr | ZTF |
| 58302.905296 | 17.315 | 0.020 | zr | ZTF |
| 58303.976812 | 17.366 | 0.020 | zr | ZTF |
| 58304.900057 | 17.345 | 0.020 | zr | ZTF |
| 58305.925703 | 17.265 | 0.020 | zr | ZTF |
| 58307.909307 | 17.256 | 0.020 | zr | ZTF |
| 58310.925378 | 17.250 | 0.020 | zr | ZTF |
| 58312.926660 | 17.273 | 0.020 | zr | ZTF |
| 58313.911299 | 17.369 | 0.020 | zr | ZTF |
| 58314.950491 | 17.323 | 0.020 | zr | ZTF |
| 58315.977540 | 17.320 | 0.020 | zr | ZTF |
| 58316.977759 | 17.568 | 0.022 | zr | ZTF |
| 58319.956010 | 17.302 | 0.020 | zr | ZTF |
| 58320.886387 | 17.273 | 0.020 | zr | ZTF |
| 58321.968707 | 17.285 | 0.020 | zr | ZTF |
| 58322.879952 | 17.298 | 0.020 | zr | ZTF |
| 58323.977180 | 17.324 | 0.020 | zr | ZTF |
| 58324.972342 | 17.252 | 0.020 | zr | ZTF |
| 58325.973499 | 17.123 | 0.019 | zr | ZTF |
| 58326.913056 | 17.301 | 0.020 | zr | ZTF |
| 58327.902385 | 17.255 | 0.020 | zr | ZTF |
| 58328.903369 | 17.257 | 0.020 | zr | ZTF |
| 58329.862278 | 17.266 | 0.020 | zr | ZTF |
| 58330.902350 | 17.256 | 0.020 | zr | ZTF |
| 58332.855901 | 17.216 | 0.019 | zr | ZTF |
| 58333.838469 | 17.232 | 0.020 | zr | ZTF |
| 58334.861190 | 17.228 | 0.019 | zr | ZTF |
| 58336.845320 | 17.176 | 0.019 | zr | ZTF |
| 58337.844439 | 17.201 | 0.019 | zr | ZTF |
| 58338.842806 | 17.097 | 0.019 | zr | ZTF |
| 58342.847013 | 17.246 | 0.020 | zr | ZTF |
| 58343.865218 | 17.271 | 0.020 | zr | ZTF |
| 58345.889428 | 17.251 | 0.020 | zr | ZTF |
| 58346.893337 | 17.275 | 0.020 | zr | ZTF |
| 58347.907281 | 17.295 | 0.020 | zr | ZTF |
| 58349.826482 | 17.305 | 0.020 | zr | ZTF |
| 58350.890578 | 17.292 | 0.020 | zr | ZTF |
| 58351.883015 | 17.359 | 0.020 | zr | ZTF |
| 58352.807218 | 17.265 | 0.020 | zr | ZTF |
| 58353.935634 | 17.288 | 0.020 | zr | ZTF |
| 58353.972140 | 17.294 | 0.020 | zr | ZTF |

| BJD−2400000 | Mag | Magerr | Filter | Obs code |
|---|---|---|---|---|
| 58354.820205 | 17.277 | 0.020 | zr | ZTF |
| 58354.928289 | 17.298 | 0.020 | zr | ZTF |
| 58355.838185 | 17.241 | 0.020 | zr | ZTF |
| 58355.969777 | 17.310 | 0.020 | zr | ZTF |
| 58356.902001 | 17.258 | 0.020 | zr | ZTF |
| 58356.964816 | 17.250 | 0.020 | zr | ZTF |
| 58357.721232 | 17.236 | 0.020 | zr | ZTF |
| 58357.913371 | 17.177 | 0.019 | zr | ZTF |
| 58358.777754 | 17.186 | 0.019 | zr | ZTF |
| 58359.829253 | 17.211 | 0.019 | zr | ZTF |
| 58359.881836 | 17.163 | 0.019 | zr | ZTF |
| 58360.816766 | 17.200 | 0.019 | zr | ZTF |
| 58361.802323 | 17.119 | 0.019 | zr | ZTF |
| 58362.821399 | 17.042 | 0.018 | zr | ZTF |
| 58363.783181 | 16.935 | 0.018 | zr | ZTF |
| 58364.820938 | 16.833 | 0.017 | zr | ZTF |
| 58365.846274 | 16.815 | 0.017 | zr | ZTF |
| 58366.845243 | 16.839 | 0.017 | zr | ZTF |
| 58367.842706 | 16.812 | 0.017 | zr | ZTF |
| 58368.843711 | 16.828 | 0.017 | zr | ZTF |
| 58369.877020 | 16.836 | 0.017 | zr | ZTF |
| 58370.914425 | 16.910 | 0.018 | zr | ZTF |
| 58371.912314 | 16.967 | 0.018 | zr | ZTF |
| 58372.866301 | 17.092 | 0.019 | zr | ZTF |
| 58373.819152 | 17.144 | 0.019 | zr | ZTF |
| 58374.829620 | 17.264 | 0.020 | zr | ZTF |
| 58375.866895 | 17.393 | 0.021 | zr | ZTF |
| 58376.853842 | 17.382 | 0.021 | zr | ZTF |
| 58377.805290 | 17.567 | 0.022 | zr | ZTF |
| 58378.895550 | 17.568 | 0.022 | zr | ZTF |
| 58379.881952 | 17.726 | 0.023 | zr | ZTF |
| 58380.829323 | 17.538 | 0.022 | zr | ZTF |
| 58382.848894 | 17.355 | 0.020 | zr | ZTF |
| 58383.807421 | 17.243 | 0.020 | zr | ZTF |
| 58384.702219 | 17.240 | 0.020 | zr | ZTF |
| 58385.769810 | 17.238 | 0.020 | zr | ZTF |
| 58386.775975 | 17.340 | 0.020 | zr | ZTF |
| 58387.928497 | 17.381 | 0.020 | zr | ZTF |
| 58388.757792 | 17.347 | 0.020 | zr | ZTF |
| 58389.756419 | 17.385 | 0.021 | zr | ZTF |
| 58390.745265 | 17.365 | 0.020 | zr | ZTF |

| BJD−2400000 | Mag | Magerr | Filter | Obs code |
|---|---|---|---|---|
| 58423.803960 | 17.126 | 0.019 | zr | ZTF |
| 58424.746871 | 17.039 | 0.018 | zr | ZTF |
| 58425.726528 | 17.019 | 0.018 | zr | ZTF |
| 58426.753001 | 16.858 | 0.018 | zr | ZTF |
| 58427.725167 | 16.871 | 0.018 | zr | ZTF |
| 58428.742714 | 16.817 | 0.017 | zr | ZTF |
| 58429.780063 | 16.835 | 0.017 | zr | ZTF |
| 58430.699369 | 16.831 | 0.017 | zr | ZTF |
| 58431.681786 | 16.915 | 0.018 | zr | ZTF |
| 58432.764282 | 16.936 | 0.018 | zr | ZTF |
| 58434.687584 | 17.066 | 0.019 | zr | ZTF |
| 58435.766280 | 17.189 | 0.019 | zr | ZTF |
| 58436.760937 | 17.203 | 0.019 | zr | ZTF |
| 58437.761438 | 17.412 | 0.021 | zr | ZTF |
| 58441.785852 | 17.398 | 0.021 | zr | ZTF |
| 58442.766302 | 17.330 | 0.020 | zr | ZTF |
| 58447.859565 | 17.263 | 0.020 | zr | ZTF |
| 58449.841391 | 17.195 | 0.019 | zr | ZTF |
| 58456.680866 | 17.289 | 0.020 | zr | ZTF |
| 58457.674324 | 17.227 | 0.019 | zr | ZTF |
| 58464.764843 | 17.209 | 0.019 | zr | ZTF |
| 58468.769639 | 17.158 | 0.019 | zr | ZTF |
| 58471.640001 | 17.212 | 0.019 | zr | ZTF |
| 58472.616227 | 17.262 | 0.020 | zr | ZTF |
| 58474.640120 | 17.235 | 0.020 | zr | ZTF |
| 58475.661492 | 17.206 | 0.019 | zr | ZTF |
| 58483.605367 | 17.329 | 0.020 | zr | ZTF |
| 58490.652402 | 17.289 | 0.020 | zr | ZTF |
| 58494.590693 | 17.250 | 0.020 | zr | ZTF |
| 58503.621107 | 17.274 | 0.020 | zr | ZTF |
| 58511.617896 | 17.197 | 0.019 | zr | ZTF |
| 58523.656203 | 17.124 | 0.019 | zr | ZTF |
| 58607.989924 | 17.200 | 0.019 | zr | ZTF |
| 58619.920705 | 16.884 | 0.018 | zr | ZTF |
| 58638.971477 | 17.197 | 0.019 | zr | ZTF |
| 58639.911234 | 17.229 | 0.019 | zr | ZTF |
| 58641.971568 | 17.199 | 0.019 | zr | ZTF |
| 58643.967052 | 17.069 | 0.019 | zr | ZTF |
| 58644.971769 | 17.133 | 0.019 | zr | ZTF |
| 58646.968751 | 17.155 | 0.019 | zr | ZTF |
| 58650.928091 | 17.175 | 0.019 | zr | ZTF |

| BJD−2400000 | Mag | Magerr | Filter | Obs code |
|---|---|---|---|---|
| 58651.933426 | 17.165 | 0.019 | zr | ZTF |
| 58652.925428 | 17.137 | 0.019 | zr | ZTF |
| 58653.948936 | 17.206 | 0.019 | zr | ZTF |
| 58654.949041 | 17.159 | 0.019 | zr | ZTF |
| 58657.901324 | 17.115 | 0.019 | zr | ZTF |
| 58663.933840 | 17.048 | 0.018 | zr | ZTF |
| 58665.947718 | 17.019 | 0.018 | zr | ZTF |
| 58666.927388 | 17.040 | 0.018 | zr | ZTF |
| 58667.967536 | 17.098 | 0.019 | zr | ZTF |
| 58668.844192 | 17.172 | 0.019 | zr | ZTF |
| 58669.928927 | 17.135 | 0.019 | zr | ZTF |
| 58670.966449 | 17.079 | 0.019 | zr | ZTF |
| 58672.972415 | 17.074 | 0.019 | zr | ZTF |
| 58674.971334 | 17.066 | 0.019 | zr | ZTF |
| 58676.973264 | 16.921 | 0.018 | zr | ZTF |
| 58677.804584 | 16.828 | 0.017 | zr | ZTF |
| 58683.924007 | 17.117 | 0.019 | zr | ZTF |
| 58686.903473 | 16.956 | 0.018 | zr | ZTF |
| 58690.878553 | 17.122 | 0.019 | zr | ZTF |
| 58693.885290 | 17.137 | 0.019 | zr | ZTF |
| 58696.884874 | 17.173 | 0.019 | zr | ZTF |
| 58699.886679 | 17.157 | 0.019 | zr | ZTF |
| 58703.938462 | 17.166 | 0.019 | zr | ZTF |
| 58712.880140 | 17.165 | 0.019 | zr | ZTF |
| 58715.871320 | 16.974 | 0.018 | zr | ZTF |
| 58718.973404 | 16.702 | 0.017 | zr | ZTF |
| 58721.951740 | 16.439 | 0.016 | zr | ZTF |
| 58724.906182 | 16.719 | 0.017 | zr | ZTF |
| 58730.907635 | 17.215 | 0.019 | zr | ZTF |
| 58733.888486 | 17.314 | 0.020 | zr | ZTF |
| 58736.928373 | 17.266 | 0.020 | zr | ZTF |
| 58743.849687 | 17.210 | 0.019 | zr | ZTF |
| 58747.908695 | 17.031 | 0.018 | zr | ZTF |
| 58757.811011 | 16.667 | 0.017 | zr | ZTF |
| 58760.793002 | 16.599 | 0.017 | zr | ZTF |
| 58763.848818 | 16.745 | 0.017 | zr | ZTF |
| 58764.655569 | 16.693 | 0.017 | zr | ZTF |
| 58765.656212 | 16.786 | 0.017 | zr | ZTF |
| 58766.654852 | 16.911 | 0.018 | zr | ZTF |
| 58767.656106 | 16.989 | 0.018 | zr | ZTF |
| 58768.656688 | 17.194 | 0.019 | zr | ZTF |

| BJD−2400000 | Mag | Magerr | Filter | Obs code |
|---|---|---|---|---|
| 58769.656610 | 17.248 | 0.020 | zr | ZTF |
| 58770.656693 | 17.285 | 0.020 | zr | ZTF |
| 58771.656925 | 17.295 | 0.020 | zr | ZTF |
| 58772.657248 | 17.275 | 0.020 | zr | ZTF |
| 58773.655881 | 17.240 | 0.020 | zr | ZTF |
| 58774.655798 | 17.204 | 0.019 | zr | ZTF |
| 58775.655921 | 17.153 | 0.019 | zr | ZTF |
| 58776.655142 | 17.170 | 0.019 | zr | ZTF |
| 58777.655576 | 17.139 | 0.019 | zr | ZTF |
| 58778.655778 | 17.186 | 0.019 | zr | ZTF |
| 58779.655585 | 17.152 | 0.019 | zr | ZTF |
| 58781.655486 | 17.100 | 0.019 | zr | ZTF |
| 58782.654596 | 17.104 | 0.019 | zr | ZTF |
| 58783.655799 | 17.103 | 0.019 | zr | ZTF |
| 58785.655449 | 17.189 | 0.019 | zr | ZTF |
| 58786.662344 | 17.154 | 0.019 | zr | ZTF |
| 58787.654701 | 17.211 | 0.019 | zr | ZTF |
| 58788.655587 | 17.160 | 0.019 | zr | ZTF |
| 58789.655963 | 17.205 | 0.019 | zr | ZTF |
| 58790.669810 | 17.184 | 0.019 | zr | ZTF |
| 58790.677657 | 17.189 | 0.019 | zr | ZTF |
| 58791.617881 | 17.161 | 0.019 | zr | ZTF |
| 58792.654260 | 17.067 | 0.019 | zr | ZTF |
| 58792.666389 | 17.158 | 0.019 | zr | ZTF |
| 58793.619273 | 17.122 | 0.019 | zr | ZTF |
| 58794.620211 | 17.145 | 0.019 | zr | ZTF |
| 58795.594805 | 17.097 | 0.019 | zr | ZTF |
| 58796.620035 | 17.156 | 0.019 | zr | ZTF |
| 58797.622127 | 17.117 | 0.019 | zr | ZTF |
| 58798.697272 | 17.194 | 0.019 | zr | ZTF |
| 58798.752734 | 17.250 | 0.020 | zr | ZTF |
| 58799.747359 | 17.241 | 0.020 | zr | ZTF |
| 58800.781068 | 17.190 | 0.019 | zr | ZTF |
| 58801.766420 | 17.135 | 0.019 | zr | ZTF |
| 58803.761762 | 17.142 | 0.019 | zr | ZTF |
| 58804.722633 | 17.041 | 0.018 | zr | ZTF |
| 58805.722078 | 17.086 | 0.019 | zr | ZTF |
| 58806.738687 | 17.095 | 0.019 | zr | ZTF |
| 58811.636094 | 16.933 | 0.018 | zr | ZTF |
| 58812.681191 | 16.806 | 0.017 | zr | ZTF |
| 58814.660737 | 16.537 | 0.016 | zr | ZTF |

| BJD−2400000 | Mag | Magerr | Filter | Obs code |
|---|---|---|---|---|
| 58819.621810 | 16.356 | 0.016 | zr | ZTF |
| 58819.665119 | 16.570 | 0.016 | zr | ZTF |
| 58820.619413 | 16.561 | 0.016 | zr | ZTF |
| 58828.784900 | 16.730 | 0.017 | zr | ZTF |
| 58830.741007 | 16.963 | 0.018 | zr | ZTF |
| 58831.595124 | 17.034 | 0.018 | zr | ZTF |
| 58833.595566 | 17.154 | 0.019 | zr | ZTF |
| 58846.619577 | 17.434 | 0.021 | zr | ZTF |
| 58329.955351 | 18.095 | 0.037 | zg | ZTF |
| 58329.955802 | 18.063 | 0.036 | zg | ZTF |
| 58333.937363 | 18.028 | 0.035 | zg | ZTF |
| 58333.937826 | 18.101 | 0.037 | zg | ZTF |
| 58338.927788 | 17.989 | 0.035 | zg | ZTF |
| 58344.893481 | 18.065 | 0.036 | zg | ZTF |
| 58350.835019 | 18.049 | 0.036 | zg | ZTF |
| 58360.891874 | 17.966 | 0.034 | zg | ZTF |
| 58363.834723 | 17.608 | 0.029 | zg | ZTF |
| 58371.875739 | 17.735 | 0.031 | zg | ZTF |
| 58430.792504 | 17.574 | 0.029 | zg | ZTF |
| 58443.683431 | 18.041 | 0.036 | zg | ZTF |
| 58443.683883 | 18.089 | 0.036 | zg | ZTF |
| 58443.684346 | 18.040 | 0.036 | zg | ZTF |
| 58443.684797 | 18.054 | 0.036 | zg | ZTF |
| 58443.685248 | 18.021 | 0.035 | zg | ZTF |
| 58443.685711 | 18.018 | 0.035 | zg | ZTF |
| 58443.708847 | 18.095 | 0.037 | zg | ZTF |
| 58327.883194 | 17.333 | 0.018 | zr | ZTF |
| 58327.883645 | 17.360 | 0.018 | zr | ZTF |
| 58328.890937 | 17.234 | 0.017 | zr | ZTF |
| 58328.892303 | 17.237 | 0.017 | zr | ZTF |
| 58330.917340 | 17.230 | 0.017 | zr | ZTF |
| 58332.893368 | 17.194 | 0.017 | zr | ZTF |
| 58332.893819 | 17.142 | 0.017 | zr | ZTF |
| 58334.899641 | 17.188 | 0.017 | zr | ZTF |
| 58334.920209 | 17.222 | 0.017 | zr | ZTF |
| 58335.915185 | 17.156 | 0.017 | zr | ZTF |
| 58335.915648 | 17.163 | 0.017 | zr | ZTF |
| 58336.901758 | 17.183 | 0.017 | zr | ZTF |
| 58336.902221 | 17.173 | 0.017 | zr | ZTF |
| 58345.868940 | 17.273 | 0.018 | zr | ZTF |
| 58353.822966 | 17.198 | 0.017 | zr | ZTF |

| BJD−2400000 | Mag | Magerr | Filter | Obs code |
|---|---|---|---|---|
| 58354.790990 | 17.271 | 0.018 | zr | ZTF |
| 58355.812999 | 17.295 | 0.018 | zr | ZTF |
| 58356.806128 | 17.259 | 0.018 | zr | ZTF |
| 58357.833274 | 17.234 | 0.017 | zr | ZTF |
| 58359.852298 | 17.210 | 0.017 | zr | ZTF |
| 58360.833804 | 17.178 | 0.017 | zr | ZTF |
| 58362.854237 | 17.065 | 0.016 | zr | ZTF |
| 58364.874169 | 16.786 | 0.015 | zr | ZTF |
| 58365.874875 | 16.783 | 0.015 | zr | ZTF |
| 58368.822321 | 16.829 | 0.015 | zr | ZTF |
| 58372.833753 | 17.050 | 0.016 | zr | ZTF |
| 58427.761452 | 16.787 | 0.015 | zr | ZTF |
| 58429.873407 | 16.800 | 0.015 | zr | ZTF |
| 58439.749845 | 17.520 | 0.020 | zr | ZTF |
| 58443.598167 | 17.319 | 0.018 | zr | ZTF |
| 58471.719037 | 17.228 | 0.017 | zr | ZTF |

## References

Henden, A. A., & Honeycutt, R. K. 1997, PASP, 109, 441
Robinson, E. L., Nather, R. E., & Patterson, J. 1978, ApJ, 219, 168
